# Supplementary material for: From Big to Small: Multi-Scale Local Planar Guidance for Monocular Depth Estimation
Source: arXiv:1907.10326 ancillary file (2021-09-23)
Supplement: Supplementary file 1 [file bts_sm.pdf]

# From Big to Small: Multi-Scale Local Planar Guidance for Monocular Depth Estimation (Supplementary Material)

Jin Han Lee, Myung-Kyu Han, Dong Wook Ko and Il Hong Suh
Department of Electronics and Computer Engineering, Hanyang University
{jinhanlee, mkhan91, pumpblack, ihsuh}@hanyang.ac.kr

## 1. Model Architecture

| **encoder** | | | | | | | |
|---|---|---|---|---|---|---|---|
| **layer** | **k** | **s** | **ch** | **in** | **out** | **input** | **note** |
| *conv1* | 7 | 2 | 3/96 | H | H/2 | input image | |
| *maxp1* | 3 | 2 | 96/96 | H/2 | H/4 | *conv1* | max pooling |
| *dblock1* | - | 1 | 96/384 | H/4 | H/4 | *maxp1* | dense block |
| *tblock1* | - | 2 | 384/192 | H/4 | H/8 | *dblock1* | transition block |
| *dblock2* | - | 1 | 192/768 | H/8 | H/8 | *tblock1* | dense block |
| *tblock2* | - | 2 | 768/384 | H/8 | H/16 | *dblock2* | transition block |
| *dblock3* | - | 1 | 384/2112 | H/16 | H/16 | *tblock2* | dense block |
| *tblock3* | - | 2 | 2112/1056 | H/16 | H/32 | *dblock3* | transition block |
| *dblock4* | - | 1 | 1056/2208 | H/32 | H/32 | *tblock3* | dense block |
| **decoder** | | | | | | | |
| **layer** | **k** | **up** | **ch** | **in** | **out** | **input** | **note** |
| *upconv5* | 3 | 2 | 2208/512 | H/32 | H/16 | *dblock4* | |
| *iconv5* | 3 | 1 | 896/512 | H/16 | H/16 | *upconv5+tblock2* | skip connection |
| *upconv4* | 3 | 2 | 512/256 | H/16 | H/8 | *iconv5* | dense features |
| *iconv4* | 3 | 1 | 448/256 | H/8 | H/8 | *upconv4+tblock1* | skip connection |
| *aspp* | - | 1 | 256/128 | H/8 | H/8 | *iconv4* | ASPP module |
| *reduc8x8* | 1 | 1 | 128/4 | H/8 | H/8 | *aspp* | $1 \times 1$ reduction |
| *lpg8x8* | - | 8 | 4/1 | H/8 | H | *reduc8x8* | local planar guidance |
| *upconv3* | 3 | 2 | 128/128 | H/8 | H/4 | *aspp* | |
| *iconv3* | 3 | 1 | 225/128 | H/4 | H/4 | *upconv3+maxp1+lpg8x8/4* | skip connection |
| *reduc4x4* | 1 | 1 | 128/4 | H/4 | H/4 | *iconv3* | $1 \times 1$ reduction |
| *lpg4x4* | - | 4 | 4/1 | H/4 | H | *reduc4x4* | local planar guidance |
| *upconv2* | 3 | 2 | 128/64 | H/4 | H/2 | *iconv3* | |
| *iconv2* | 3 | 1 | 161/64 | H/2 | H/2 | *upconv2+conv1+lpg4x4/2* | skip connection |
| *reduc2x2* | 1 | 1 | 64/4 | H/2 | H/2 | *iconv2* | $1 \times 1$ reduction |
| *lpg2x2* | - | 2 | 4/1 | H/2 | H | *reduc2x2* | local planar guidance |
| *upconv1* | 3 | 2 | 64/32 | H/2 | H | *iconv2* | |
| *iconv1* | 3 | 1 | 35/32 | H | H | *upconv1+lpg8x8+lpg4x4+lpg2x2* | |
| *depth* | 3 | 1 | 32/1 | H | H | *iconv1* | final depth estimation |

Table 1: The proposed network architecture. From left to right, **layer**: name of the layer, **k**: kernel size, **s**: stride in convolution layers, **up**: upsampling ratio in *upconv*, **ch**: number of channels in input/output, **in** and **out**: spatial resolution of the input and output, **input**: input of the layer.

We show the structure of the proposed network architecture in Table 1. *dblock* and *tblock* are dense block and transition block with initial number of filters 96, growth rate 48 and reduction 0.5 from *DenseNet161* [1]. The output from layer *upconv4* is the dense features we define in the paper. *aspp* is the atrous spatial pyramid pooling layer [2]. "+" and "/x" operations in **input** field denote concatenation and nearest neighbor downsampling with ratio x, respectively. As it can be seen from the table, the only additional trainable parameters required for the proposed LPG layers are the kernel weights and biases in *reduc8x8*, *reduc4x4* and *reduc2x2*.

## 2. More Qualitative Results from NYU Depth V2 Test Split

We also provide more qualitative results from NYU Depth V2 test split in Figures 1-6. As we describe in the manuscript, outputs from *lpg8x8* layer tend to show the global 3D shape of the scenes while outputs from *lpg2x2* and *lpg4x4* show finer details that are additive together with the outputs from the other LPG layers to get the final depth estimation.

## 3. Qualitative Results from a sequence of KITTI Dataset

Finally, we attach a video showing our depth estimation results on a sequence of the KITTI Eigen test split (*2011_10_03_drive_0027*, no frames in the sequence are used for the training). Compared to the existing works, we can see that the proposed method produces much clearer results especially on object boundaries.

## References


[1] G. Huang, Z. Liu, L. Van Der Maaten, and K. Q. Weinberger. Densely connected convolutional networks. In *CVPR*, volume 1, page 3, 2017. 2

[2] M. Yang, K. Yu, C. Zhang, Z. Li, and K. Yang. Denseaspp for semantic segmentation in street scenes. In *Proceedings of the IEEE Conference on Computer Vision and Pattern Recognition*, pages 3684–3692, 2018. 2

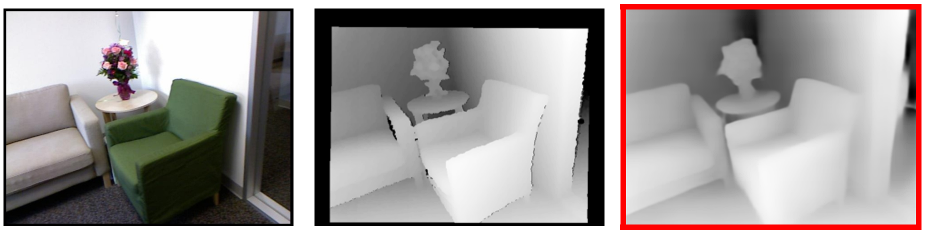

(a) Input (b) Ground truth (c) Estimated depth map

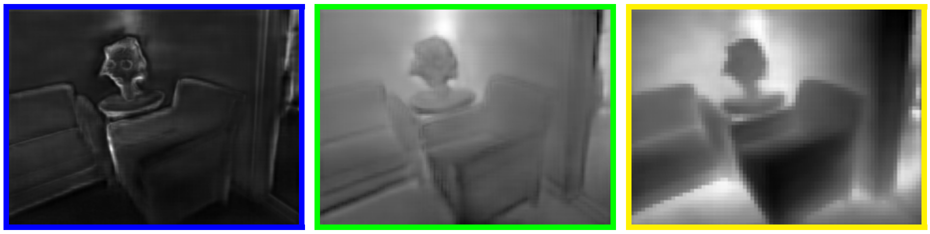

(d) Output from *lpg2x2* (e) Output from *lpg4x4* (f) Output from *lpg8x8*

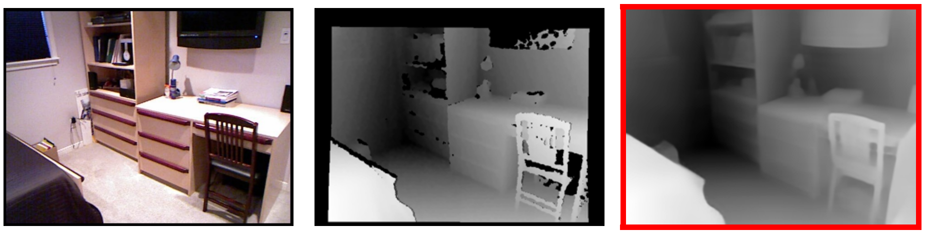

(a) Input (b) Ground truth (c) Estimated depth map

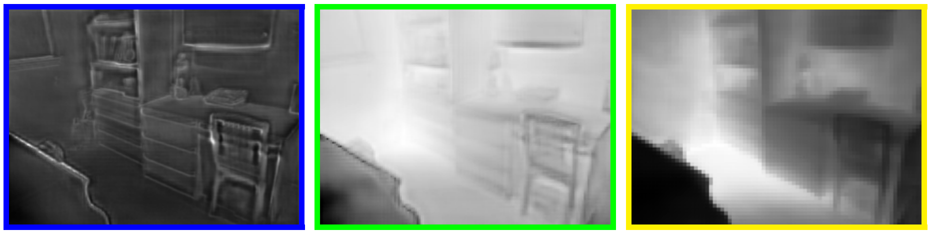

(d) Output from *lpg2x2* (e) Output from *lpg4x4* (f) Output from *lpg8x8*

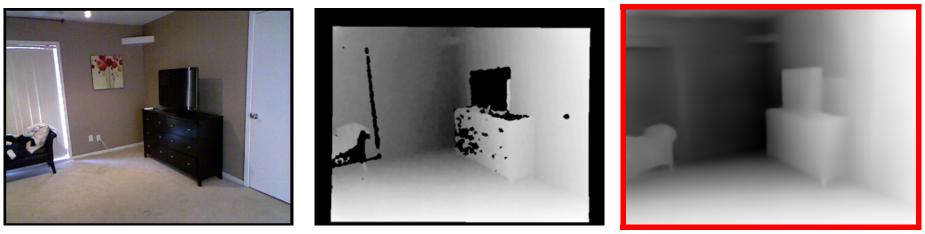

(a) Input (b) Ground truth (c) Estimated depth map

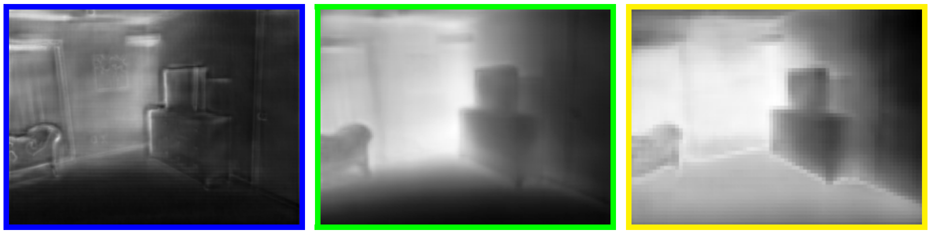

(d) Output from *lpg2x2* (e) Output from *lpg4x4* (f) Output from *lpg8x8*

Figure 1: **Qualitative results on the NYU Depth V2 test split with outputs from the proposed LPG layers.**

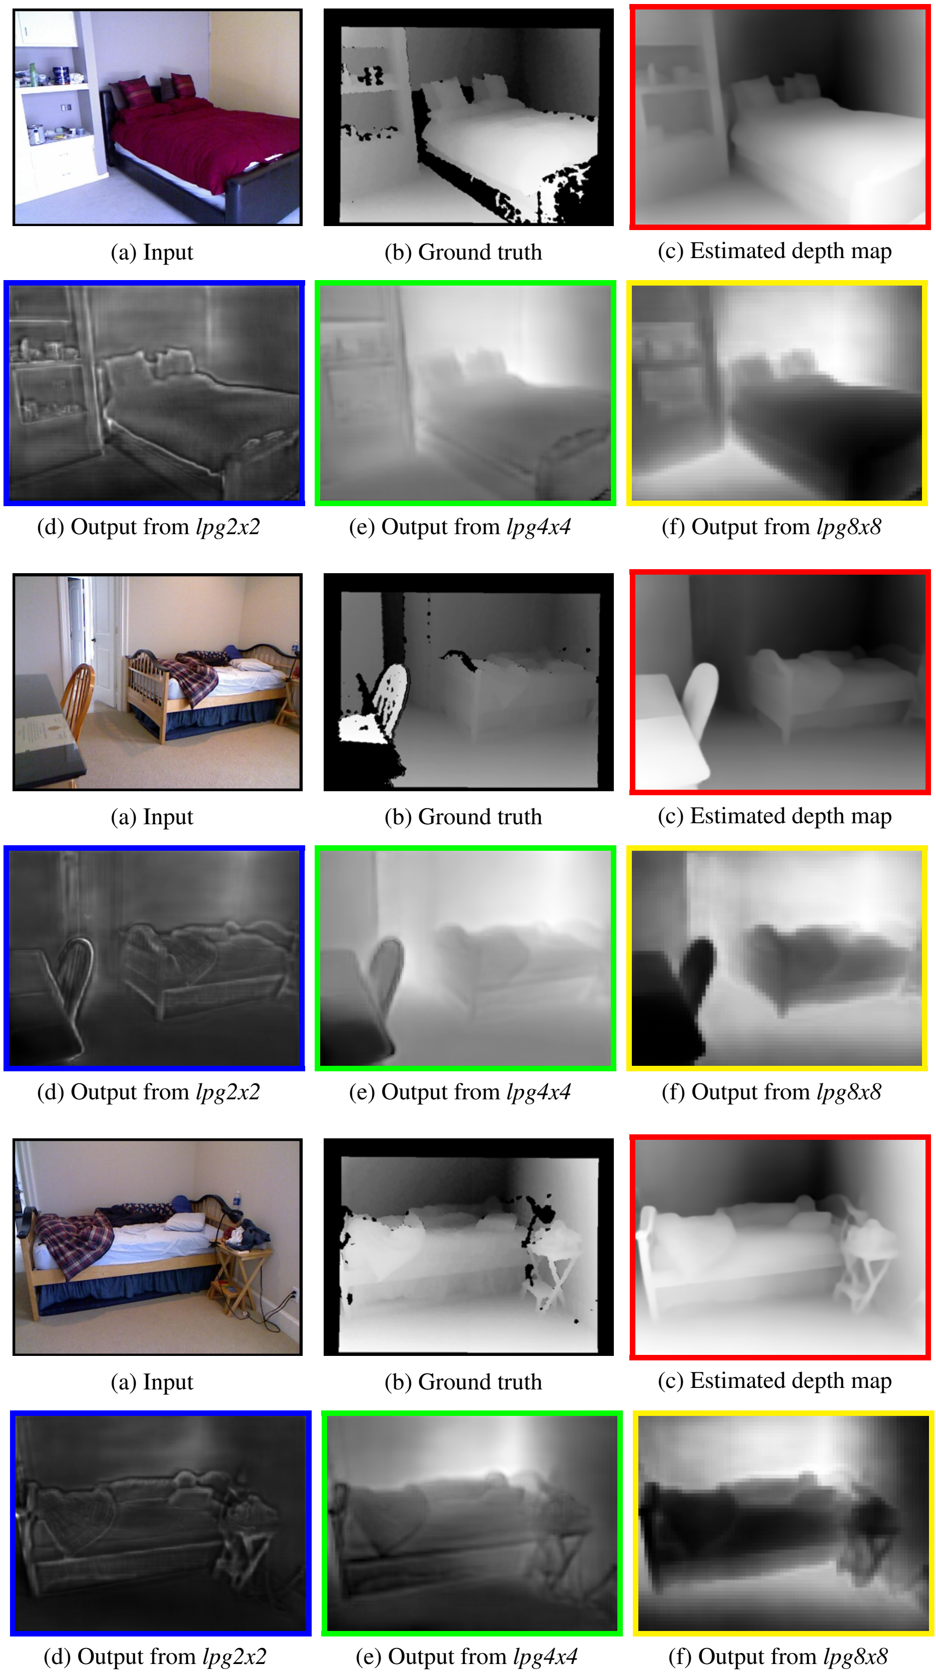

(a) Input (b) Ground truth (c) Estimated depth map

(d) Output from *lpg2x2* (e) Output from *lpg4x4* (f) Output from *lpg8x8*

(a) Input (b) Ground truth (c) Estimated depth map

(d) Output from *lpg2x2* (e) Output from *lpg4x4* (f) Output from *lpg8x8*

(a) Input (b) Ground truth (c) Estimated depth map

(d) Output from *lpg2x2* (e) Output from *lpg4x4* (f) Output from *lpg8x8*

Figure 2: **Qualitative results on the NYU Depth V2 test split with outputs from the proposed LPG layers.**

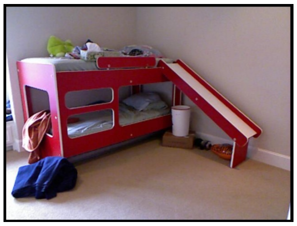
(a) Input

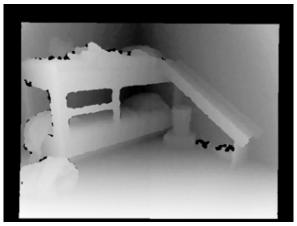
(b) Ground truth

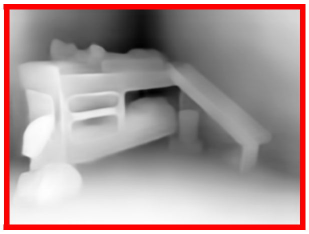
(c) Estimated depth map

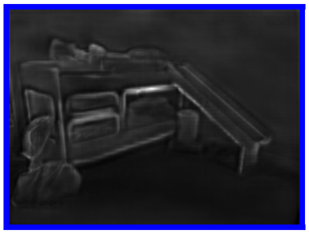
(d) Output from *lpg2x2*

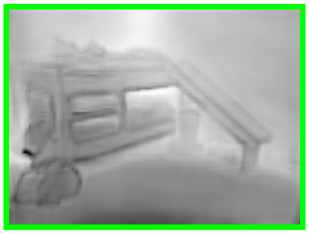
(e) Output from *lpg4x4*

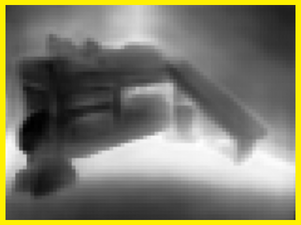
(f) Output from *lpg8x8*

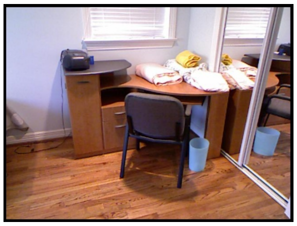
(a) Input

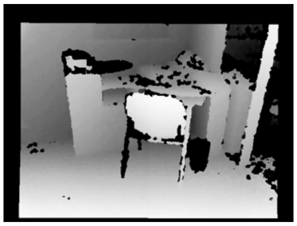
(b) Ground truth

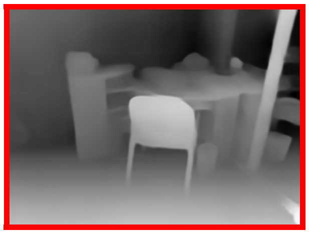
(c) Estimated depth map

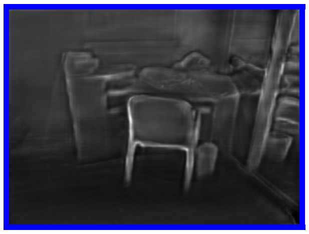
(d) Output from *lpg2x2*

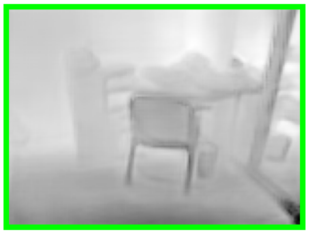
(e) Output from *lpg4x4*

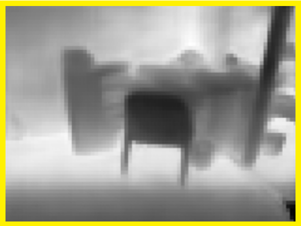
(f) Output from *lpg8x8*

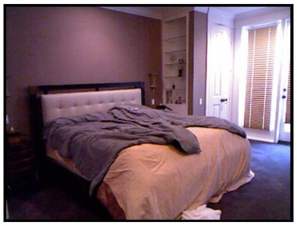
(a) Input

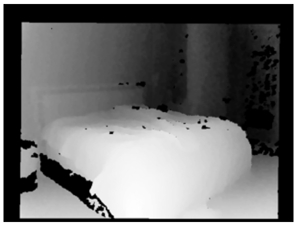
(b) Ground truth

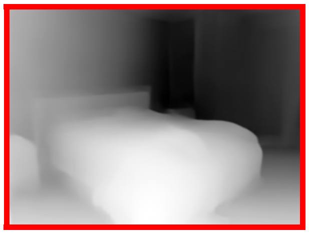
(c) Estimated depth map

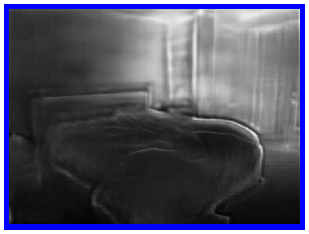
(d) Output from *lpg2x2*

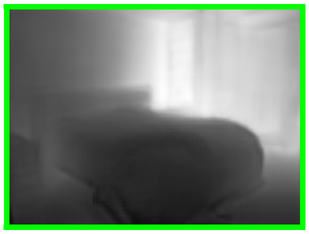
(e) Output from *lpg4x4*

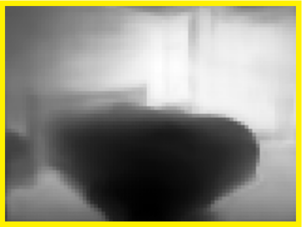
(f) Output from *lpg8x8*

Figure 3: **Qualitative results on the NYU Depth V2 test split with outputs from the proposed LPG layers.**

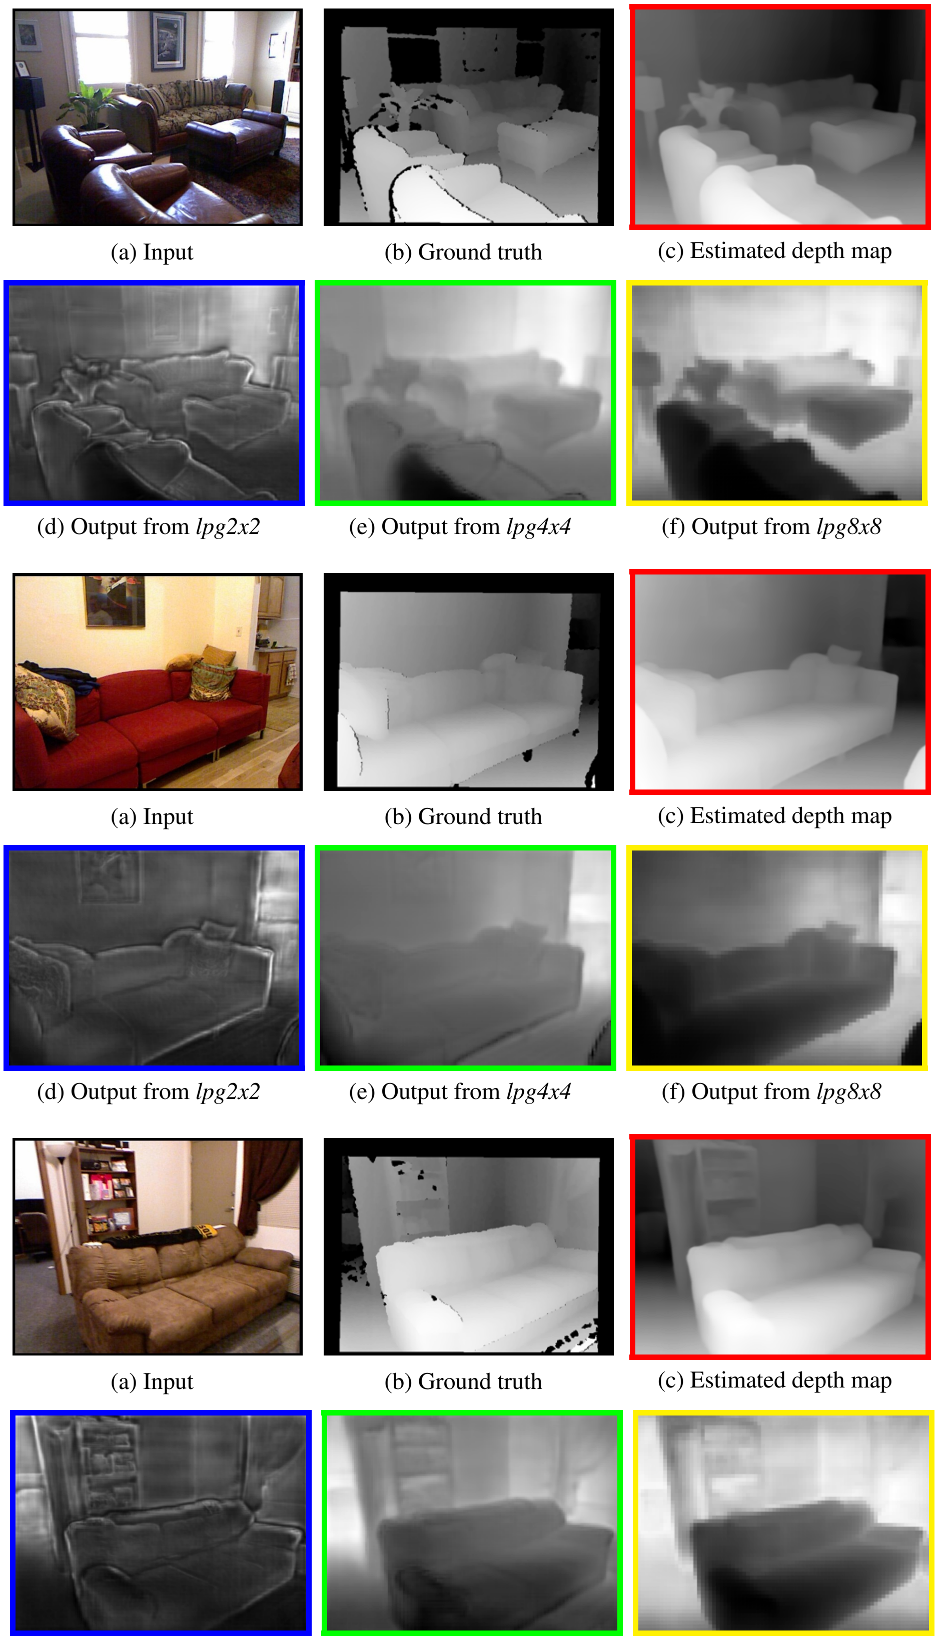

(a) Input (b) Ground truth (c) Estimated depth map

(d) Output from *lpg2x2* (e) Output from *lpg4x4* (f) Output from *lpg8x8*

(a) Input (b) Ground truth (c) Estimated depth map

(d) Output from *lpg2x2* (e) Output from *lpg4x4* (f) Output from *lpg8x8*

(a) Input (b) Ground truth (c) Estimated depth map

(d) Output from *lpg2x2* (e) Output from *lpg4x4* (f) Output from *lpg8x8*

Figure 4: **Qualitative results on the NYU Depth V2 test split with outputs from the proposed LPG layers.**

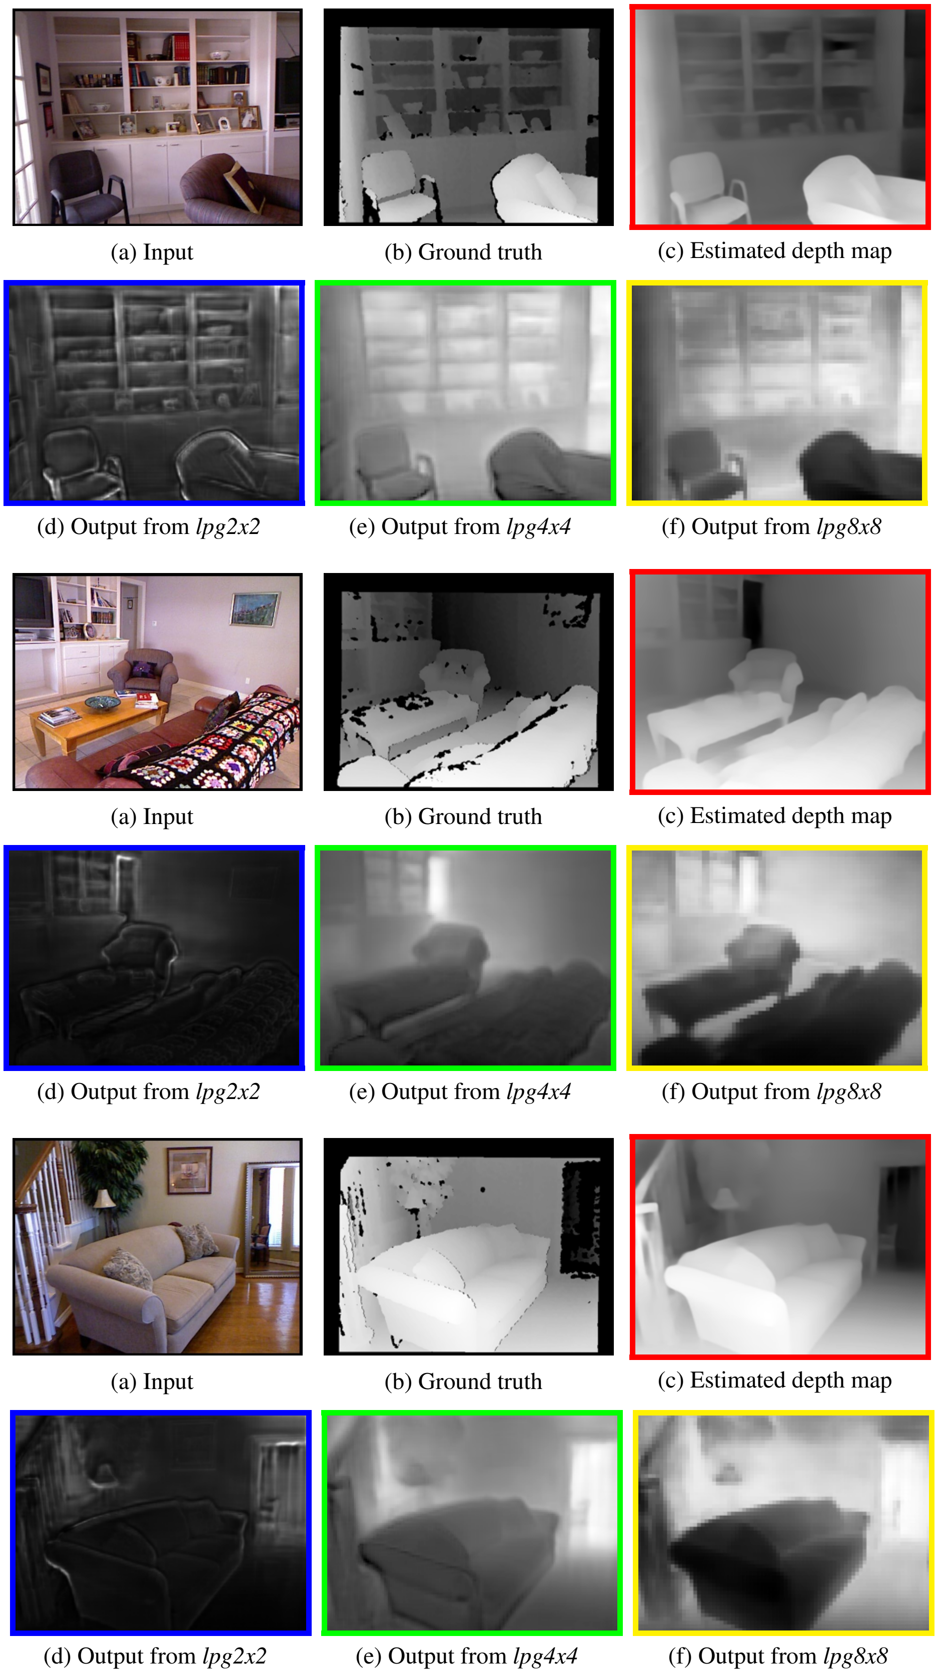

(a) Input (b) Ground truth (c) Estimated depth map

(d) Output from *lpg2x2* (e) Output from *lpg4x4* (f) Output from *lpg8x8*

(a) Input (b) Ground truth (c) Estimated depth map

(d) Output from *lpg2x2* (e) Output from *lpg4x4* (f) Output from *lpg8x8*

(a) Input (b) Ground truth (c) Estimated depth map

(d) Output from *lpg2x2* (e) Output from *lpg4x4* (f) Output from *lpg8x8*

Figure 5: **Qualitative results on the NYU Depth V2 test split with outputs from the proposed LPG layers.**

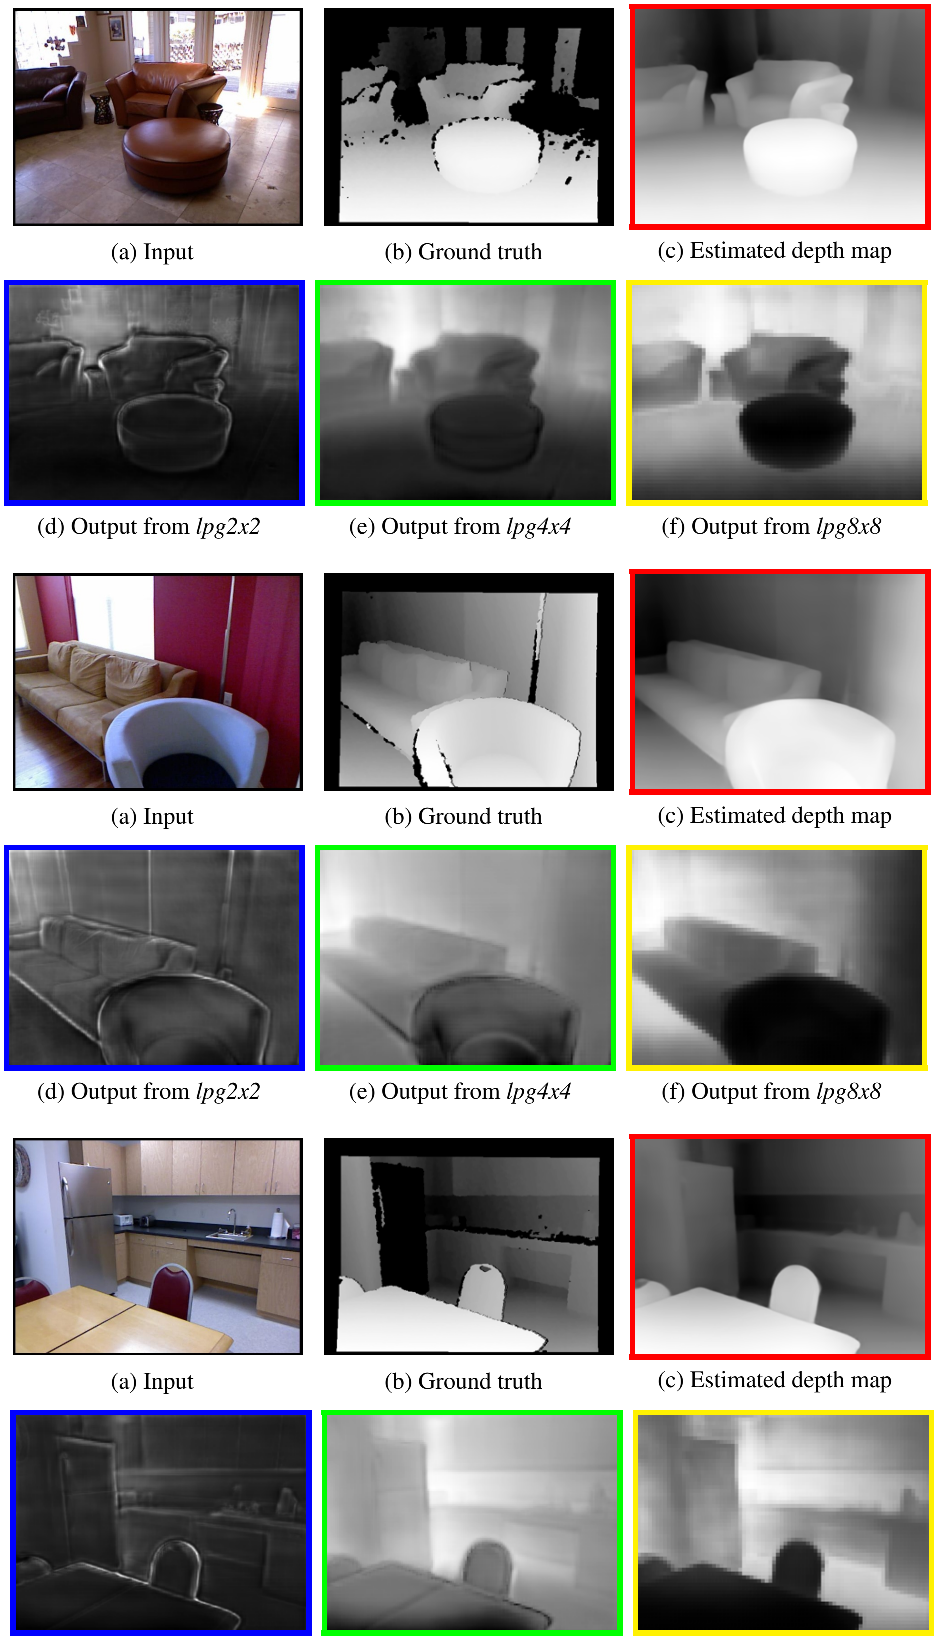

(a) Input (b) Ground truth (c) Estimated depth map

(d) Output from *lpg2x2* (e) Output from *lpg4x4* (f) Output from *lpg8x8*

(a) Input (b) Ground truth (c) Estimated depth map

(d) Output from *lpg2x2* (e) Output from *lpg4x4* (f) Output from *lpg8x8*

(a) Input (b) Ground truth (c) Estimated depth map

(d) Output from *lpg2x2* (e) Output from *lpg4x4* (f) Output from *lpg8x8*

Figure 6: **Qualitative results on the NYU Depth V2 test split with outputs from the proposed LPG layers.**
